# Supplementary material for: MIMAFace: Face Animation via Motion-Identity Modulated Appearance Feature Learning
Source: arXiv:2409.15179 source file (2024-09-23)
Supplement: Supplementary file 1 [file supp.tex]

% CVPR 2024 Paper Template; see https://github.com/cvpr-org/author-kit

\documentclass[11pt,twocolumn,letterpaper]{article}

%%%%%%%%% PAPER TYPE  - PLEASE UPDATE FOR FINAL VERSION
\usepackage{cvpr}              % To produce the CAMERA-READY version
% \usepackage[review]{cvpr}      % To produce the REVIEW version
% \usepackage[pagenumbers]{cvpr} % To force page numbers, e.g. for an arXiv version

% Import additional packages in the preamble file, before hyperref
\input{preamble}

% It is strongly recommended to use hyperref, especially for the review version.
% hyperref with option pagebackref eases the reviewers' job.
% Please disable hyperref *only* if you encounter grave issues, 
% e.g. with the file validation for the camera-ready version.
%
% If you comment hyperref and then uncomment it, you should delete *.aux before re-running LaTeX.
% (Or just hit 'q' on the first LaTeX run, let it finish, and you should be clear).
\definecolor{cvprblue}{rgb}{0.21,0.49,0.74}
\usepackage[pagebackref,breaklinks,colorlinks,citecolor=cvprblue]{hyperref}
\usepackage{algorithm}
\usepackage{algorithmic}
\usepackage{multirow}
\usepackage{csquotes}
\usepackage{color}% http://ctan.org/pkg/color
\usepackage{hyperref} 
\hypersetup{ 
 colorlinks=true, 
 linkcolor=black, 
 } 

% \usepackage[linkbordercolor={0 0 1}]{hyperref}

%%%%%%%%% PAPER ID  - PLEASE UPDATE
 % *** Enter the Paper ID here

%%%%%%%%% TITLE - PLEASE UPDATE
%\title{Unifying Top-down and Bottom-up Human Scanpath Prediction with Transformer}
\title{Unifying Top-down and Bottom-up Scanpath Prediction Using Transformers\\
\vspace{0.5em}{\it Supplementary Material}}
% Minh: I remove Human from the title. Should we put it back? 

%%%%%%%%% AUTHORS - PLEASE UPDATE
\author{Zhibo Yang\textsuperscript{1,2}, Sounak Mondal\textsuperscript{1}, Seoyoung Ahn\textsuperscript{1}, Ruoyu Xue\textsuperscript{1}, \\  Gregory Zelinsky\textsuperscript{1}, Minh Hoai\textsuperscript{1,3}, Dimitris Samaras\textsuperscript{1} \\
\textsuperscript{1}Stony Brook University~~~  \textsuperscript{2}Waymo LLC~~~
\textsuperscript{3}VinAI Research
}

\begin{document}
\input{definitions}
\maketitle
\tableofcontents
\input{sec/X_suppl}
{
    \small
    \bibliographystyle{ieeenat_fullname}
    \bibliography{main}
}

\end{document}
